# Supplementary material for: Reconfigurable flat bands from cooperative moir\'e and charge order
Source: arXiv:2511.05648 source file (2026-08-11)
Supplement: Supplementary file 1 [file supp.pdf]

# Supplementary Materials for
# Flat electronic bands from cooperative moiré and charge order

B.K. Saika,[1,*] S. Buchberger,[1,*] S. Mo,[1] A. Rajan,[1] D. Halliday,[1,2] Y.-C. Yao,[1,3]
L.C. Rhodes,[1] B. Sarpi,[2] T. Balasubramanian,[4] C. Polley,[4] P. Wahl,[1] and P.D.C. King[1,†]

[1]*SUPA, School of Physics and Astronomy, University of St Andrews, St Andrews KY16 9SS, United Kingdom*
[2]*Diamond Light Source, Harwell Science and Innovation Campus, Didcot, OX11 0DE, United Kingdom*
[3]*Max Planck Institute for Chemical Physics of Solids, Nöthnitzer Strasse 40, Dresden 01187, Germany*
[4]*MAX IV Laboratory, Lund University, Lund, Sweden*

(Dated: November 7, 2025)

## MATERIALS AND METHODS

### Molecular beam epitaxy

Monolayer $TiSe_2$ films were grown by molecular beam epitaxy (MBE) in a DCA R450 MBE growth reactor on natural graphite crystals purchased from *NGS Natugraphit* and on 1 mm thick highly oriented pyrolytic graphite (HOPG) substrates purchased from *MaTeck*. For easier handling, the natural graphite crystals were glued onto 1 mm thin tantalum foil chips using high-temperature carbon paste from Agar Scientific. The glue was outgassed at $> 600°$C under $\sim 1 \times 10^{-7}$ mbar vacuum in a separate annealing chamber. The substrates were cleaved in air using adhesive tape to expose a fresh surface and loaded immediately into the load lock of the growth vacuum system, where they were degassed at 200°C for 10 h. Directly before the film growth, the substrates were annealed at 750°C for 30 minutes.

All samples were grown using a nucleation-assisted MBE growth mode as introduced in Refs. [59,60]. The films for photoemission measurements were grown on natural graphite, using a growth temperature of 550°C. 3N5 pure Ti was evaporated from a high-temperature effusion cell at a cell temperature of 1455°C. A valved cracker cell was used for the evaporation of 5N pure Se. The base of the cell was held at a temperature of 163°C and the cracking zone at 500°C to produce a supply of Se monomers and dimers with a beam-equivalent pressure of $2 \times 10^{-7}$ mbar. The low Ti supply used for the growth hinders the accurate determination of the Ti beam-equivalent pressure, but it is estimated to be at least two orders of magnitude lower than the Se supply. For an enhanced nucleation rate [59], 5N pure Ge was co-evaporated from a FOCUS EFM electron beam evaporator with a flux of 1.0 nA as measured by the integrated flux monitor. With this method, a near-complete monolayer film was deposited within a growth time of 1 h. To end the growth, the supply of Ti and Ge was cut off and the sample temperature was ramped down at a rate of 20 K/min under Se flux to avoid excessive Se vacancy formation. The Se supply was cut off at 260°C. To protect the samples during the transport to the synchrotron, they were capped with a $\sim$ 5 nm thick amorphous Se layer, deposited at room temperature. The samples were then taken out of the vacuum system and transferred to the beamline. At the Max-IV synchrotron, the samples were decapped by annealing them at 260°C under $\sim 10^{-10}$ mbar vacuum for 1 h in a preparation chamber connected to the measurement chamber.

HOPG substrates were used for the samples for scanning tunnelling microscopy (STM) and micro-focus low-energy electron diffraction ($\mu$-LEED). For the STM data shown here, the enhanced nucleation was achieved by pre-sputtering the substrate with He ions [60], (partial pressure: $5.6 \times 10^{-7}$ mbar), using an accelerating voltage of 200 V and for a duration of 30 s. In turn, no Ge was co-evaporated during the growth. A slightly shorter growth time of 55 min was used, while all remaining growth parameters were as described above for the photoemission samples. We also fabricated samples using the Ge-assisted growth method without additional pre-sputtering, achieving very similar results. For the samples for $\mu$-LEED, we used a growth temperature of 600°C, Ti cell temperature of 1460°C, Se beam equivalent pressure of $2 \times 10^{-7}$ mbar, a Ge flux of 1.0 nA for assisted nucleation and a growth time of 57 minutes. The samples were transferred from the growth chamber to the STM and $\mu$-LEED measurement chambers under ultra-high vacuum, using vacuum suitcases.

### Angle-resolved photoemission

ARPES experiments were performed at the Bloch endstation (A-branch) of the MAX IV synchrotron, Sweden, using a Scienta DA30 electron analyser. The utilised photon energies and light polarisations are noted in the figure captions, and the sample

* These authors contributed equally
† pdk6@st-andrews.ac.uk

was kept at the base temperature of $T = 18$ K throughout. The light spot size on the sample was $\approx 10$ $\mu$m $\times$ $15$ $\mu$m. Surface dosing was performed in the analysis chamber using a SAES Rb alkali dispenser held at a current of 4.5 A, with the sample held at 18 K. The current on the source was ramped up before the sample was rotated to face the doser, with a deposition time of 5 s as measured from the point at which the sample was directly facing the source. The carrier densities of pristine and dosed samples were determined from a Luttinger analysis of their measured Fermi surfaces. The carrier densities of pristine samples were found to be in the range 0.03-0.04 $e^-$ per Ti atom. After a single 5 s dose of Rb deposition, these increased to 0.08-0.09 $e^-$ per Ti atom. In addition, we performed a second dosing of 30 s for the data shown in Supplementary Fig. S3, from which we estimate a carrier density of 0.14 $e^-$ per Ti atom. ARPES data analysis was performed using the *peaks* package [65] .

### Scanning tunelling microscopy

In situ STM measurements were performed using a home-built STM which operates in cryogenic ultra-high vacuum at temperature of $1.8$ K. From the vacuum suitcase, the samples are transferred to an ultra-high vacuum chamber connected to the STM with typical pressures no larger than $5 \times 10^{-9}$ mbar before being inserted into the cryogenic vacuum of the STM chamber. The STM tip was made of Pt-Ir wire and prepared on a Au$(111)$ surface by field emission prior to the measurements. The bias voltage is applied to the sample with the tip at virtual ground. All topographies were taken in constant current mode.

### Low-energy electron diffraction

$\mu$-LEED experiments were conducted at the I06-2 offline laser-PEEM/LEEM (photoemission/low energy electron microscope) instrument at Diamond Light Source, UK. The room-temperature $\mu$-LEED data was measured from a single HOPG domain as determined from dark-field imaging. The $\mu$-LEED measurements were performed using a 10 $\mu$m illumination aperture, a high voltage of 12 kV and a start voltage of 22 V.

## SECTION I: MOIRÉ LATTICE SIMULATIONS

The construction of the moiré lattice used to define the expected Bragg spots in Fig. 2(b,e) of the main text was performed by considering the product of periodic functions which give rise to the beating frequencies of the moiré pattern, following the method described by Zeller and Günther [40]. We use a simple cosine lattice function

$$f = \frac{1}{9} + \frac{8}{9}\prod_{i=1}^{3}\cos\left(\mathbf{b_i}\cdot\mathbf{r}\right) \tag{S1}$$

where $\mathbf{b}_\mathrm{i}$ are the reciprocal lattice vectors ($i = 1, 2, 3$). Higher harmonics can be included by considering higher orders of the expression. The product of two lattice functions with different periodicities will then contain the moiré pattern arising from the interference between the two cosine functions.

Taking $\mathbf{b}_\mathrm{i}^{\mathbf{TiSe_2}}$ and $\mathbf{b}_\mathrm{i}^{\mathbf{Gr}}$ as the reciprocal lattice vectors of $TiSe_2$ and graphite, we define the lattice functions using Eq. S1:

$$f_{\mathrm{TiSe_2}} = \frac{1}{9} + \frac{8}{9}\cos\left(\mathbf{b_1}^{\mathrm{TiSe_2}}\cdot\mathbf{r}\right)\cos\left(\mathbf{b_2}^{\mathrm{TiSe_2}}\cdot\mathbf{r}\right)\cos\left(\mathbf{b_3}^{\mathrm{TiSe_2}}\cdot\mathbf{r}\right), \tag{S2}$$

$$f_{\mathrm{Gr}} = \frac{1}{9} + \frac{8}{9}\cos\left(\mathbf{b_1}^{\mathrm{Gr}}\cdot\mathbf{r}\right)\cos\left(\mathbf{b_2}^{\mathrm{Gr}}\cdot\mathbf{r}\right)\cos\left(\mathbf{b_3}^{\mathrm{Gr}}\cdot\mathbf{r}\right), \tag{S3}$$

$$f_{\mathrm{CDW}} = \frac{5}{9} + \frac{4}{9}\cos\left(\mathbf{b_1}^{\mathrm{CDW}}\cdot\mathbf{r}\right)\cos\left(\mathbf{b_2}^{\mathrm{CDW}}\cdot\mathbf{r}\right)\cos\left(\mathbf{b_3}^{\mathrm{CDW}}\cdot\mathbf{r}\right), \tag{S4}$$

where we also define the charge-density wave (CDW) periodic function within the same framework, but using a smaller value for the amplitude of the modulation. By multiplying the lattice functions and taking the Fourier transform, we can produce the frequencies expected by the moiré intereference.

Supplementary Fig. S1 shows the real space and corresponding FFT images of the constructed lattice functions. In Supplementary Fig. S1(a), the $TiSe_2$ lattice is displayed in the normal phase, using $f^2_{\mathrm{TiSe_2}}$ to include the second-order harmonics. The addition of the CDW is shown in Supplementary Fig. S1(b), where we multiply the normal state $f^2_{\mathrm{TiSe_2}}$ with the function $f_{\mathrm{CDW}}$, producing the expected $2 \times 2$ modulation in real space with the corresponding half-order peaks in reciprocal space. The

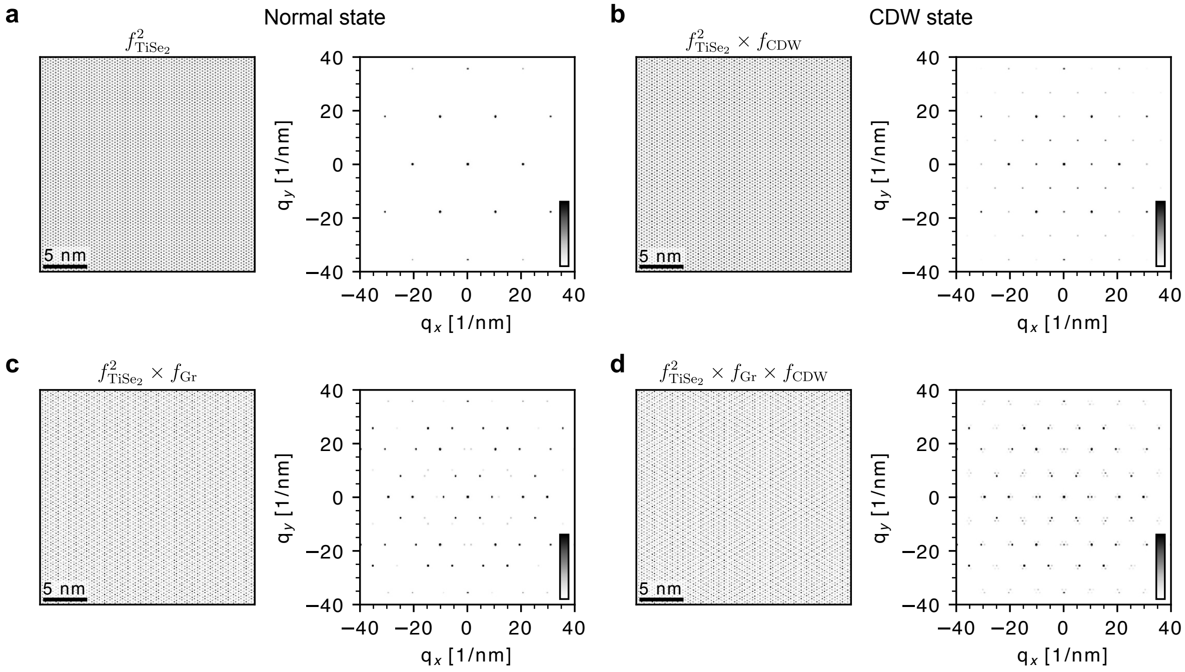


Supplementary Fig. S1. **Moiré lattice simulation.** Real-space (left) and FFT images (right) of the constructed (a) normal state of $TiSe_2$, with the inclusion of the second harmonic lattice function $f^2_{\mathrm{TiSe_2}}$ and (b) CDW state of $TiSe_2$, additionally including the CDW modulation $f_{\mathrm{CDW}}$. Corresponding simulations of (c) the $TiSe_2$/gr moiré in the normal state and (d) in the CDW state.

simulation of the lattice moiré pattern in $TiSe_2$/Gr. is shown in Supplementary Fig. S1(c), in which $f^2_{\mathrm{TiSe_2}} \times f_{\mathrm{Gr}}$ produces the incommensurate $\mathbf{q}_m^{lat}$ peaks in reciprocal space related to the differences of the lattice parameters. Additionally including the CDW modulation produces a long wavelength moiré modulation as shown in Supplementary Fig. S1(d), consistent with our experimental findings reported in the main text.

## SECTION II: EDC FITTING

In order to determine the bandwidth of the flat, topmost valence band branch, a series of EDCs across the valence band top around the M point of $TiSe_2$ were fit with a model of two Doniach-Sunjic (DS) line profiles and a linear background (see Supplementary Fig. S2 (a)). DS profiles were used to account for the asymmetric peak shape which is observed in the experimental data. Such fits were conducted across the full Brillouin zone of the CDW-moiré lattice ($-\mathbf{q}_{\mathrm{m}}^{\mathrm{CDW}}/2$ to $\mathbf{q}_{\mathrm{m}}^{\mathrm{CDW}}/2$ from the M point, see example fits in Supplementary Fig. S2 (b)). The extracted peak positions across the Brillouin zone are shown in Supplementary Fig. S2 (c), demonstrating the extremely flat nature of the topmost valence band state (with an upper limit on the bandwidth of 2 meV extracted here). The statistical errors of the curve fits are smaller than the symbol size in Supplementary Fig. S2 (c), and likely underestimate the uncertainty of the obtained band positions due to systematic errors in our photoemission experiments. Using different fitting models, we obtained slight deviations in the obtained peak positions. While the model shown in Supplementary Fig. S2 gave the best fit to the data, we use the variation in bandwidth obtained from these different fitting models to provide an estimate of the error on the bandwidth, as quoted in the main text.

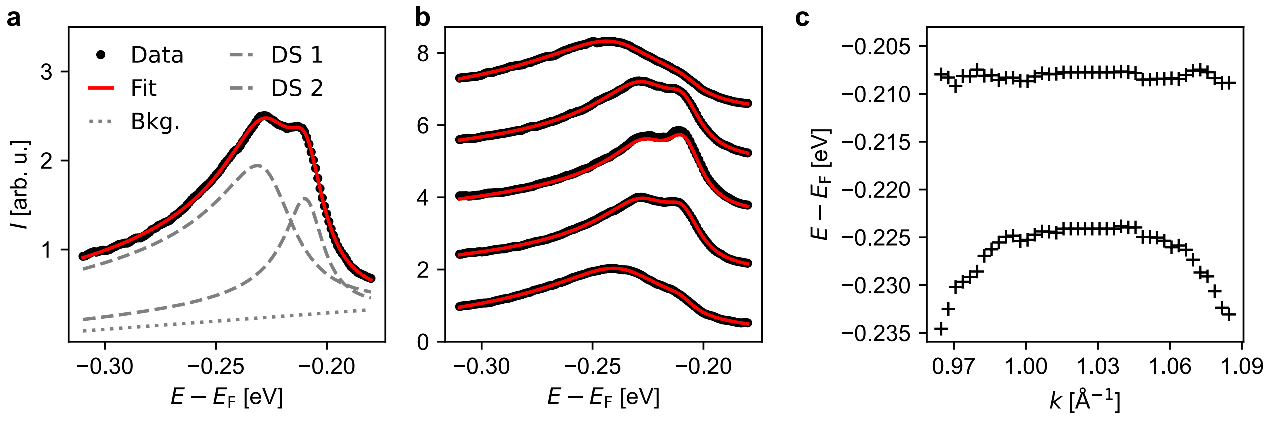


Supplementary Fig. S2. **EDC fitting.** (a) Example fit of an EDC with two Doniach-Sunjic line profiles (DS1 and DS2) and linear background. The model components are shown as grey lines. (b) Example EDCs and best fits across the CDW-moiré Brillouin zone at (-0.5, -0.25, 0, 0.25, 0.5) $\times\mathbf{q}_{\mathrm{m}}^{\mathrm{CDW}}$ from the M point of $TiSe_2$. (c) Peak positions of the two peaks across the full CDW-moiré Brillouin zone.

## SECTION III: CONTINUUM MODEL OF THE ELECTRONIC STRUCTURE

### Effective model

The low-energy electronic structure of $TiSe_2$ in the CDW state was calculated using an effective 5-band model which takes into account the momentum-selective hybridization between the Se-$p$ and Ti-$d$ bands [41]:

$$H_0(\mathbf{k}) = \begin{bmatrix} e_1 & 0 & 0 & \Delta\cos(\theta) & \Delta\sin(\theta) \\ 0 & e_2 & 0 & \Delta\cos(\theta-2\pi/3) & \Delta\sin(\theta-2\pi/3) \\ 0 & 0 & e_3 & \Delta\cos(\theta-4\pi/3) & \Delta\sin(\theta-4\pi/3) \\ \Delta\cos(\theta) & \Delta\cos(\theta-2\pi/3) & \Delta\cos(\theta-4\pi/3) & h_1 & i\lambda_{SOC} \\ \Delta\sin(\theta) & \Delta\sin(\theta-2\pi/3) & \Delta\sin(\theta-4\pi/3) & -i\lambda_{SOC} & h_2 \end{bmatrix} \tag{S5}$$

where $\Delta$ and $\lambda_{SOC}$ represent the CDW hybridisation and the spin-orbit coupling strength, respectively. The orbital-selective hybridisation is encoded in the angle $\theta = \tan^{-1}(k_y/k_x)$. The diagonal terms describe anisotropic parabolic bands derived from the normal-state electronic structure:

$$e_1 = e_c + \mu(k_x^2 + k_y^2) \tag{S6}$$

$$e_2 = e_c + \mu\left(-\frac{1}{2}k_x + \frac{\sqrt{3}}{2}k_y\right)^2 + \nu\left(-\frac{\sqrt{3}}{2}k_x - \frac{1}{2}k_y\right)^2 \tag{S7}$$

$$e_3 = e_c + \mu\left(-\frac{1}{2}k_x - \frac{\sqrt{3}}{2}k_y\right)^2 + \nu\left(\frac{\sqrt{3}}{2}k_x - \frac{1}{2}k_y\right)^2 \tag{S8}$$

$$h_1 = e_h - \mu_{inner}(k_x^2 + k_y^2) \tag{S9}$$

$$h_2 = e_h - \mu_{outer}(k_x^2 + k_y^2) \tag{S10}$$

where $\mu$ and $\nu$ are parameters related to the inverse effective mass and encode the ellipticity of $TiSe_2$'s conduction pockets, whereas $\mu_{inner}$ and $\mu_{outer}$ relate to the inverse effective mass of the inner and outer hole bands.

To estimate the effective model parameters used for the calculations shown in the main text, we first constrain our parameters to fit the measured band structure in the normal state. To reduce the contribution from fluctuations of the CDW correlations which are thought to contribute to the opening of a band gap in the electronic structure even above $T_{\mathrm{CDW}}$ [50], we use ARPES

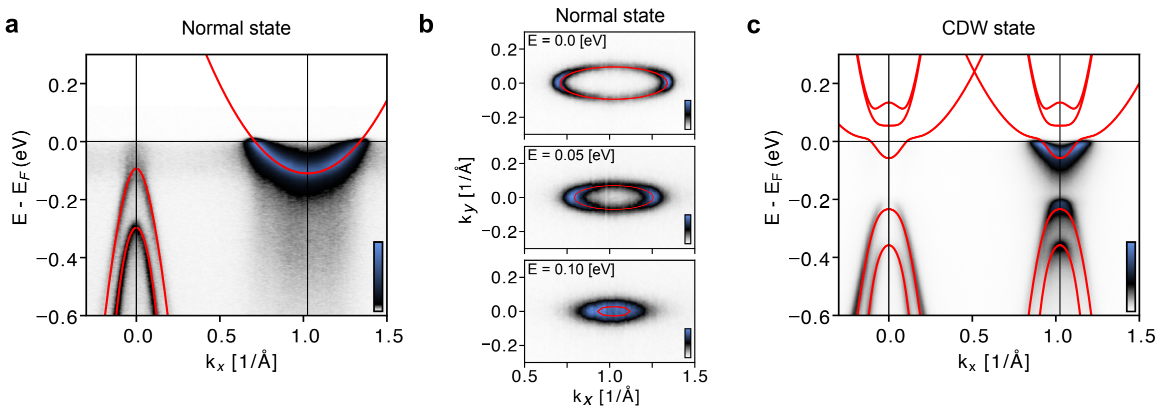


Supplementary Fig. S3. **Charge density wave model.** (a) Normal state version of the five band model in Eq. S5, superimposed on the normal state band structure of Rb-dosed sample as measured by ARPES ($h\nu = 80$ eV, LV-polarisation, $T = 18$ K, 30 s Rb dosing). (b) Constant-energy maps ($h\nu = 49$ eV, LV-polarisation, $T = 18$ K) in the normal state overlaid with the calculated energy contours of the elliptical electron pocket. (c) Five band model constrained to the normal state but with CDW hybridisation strength $\Delta = 150$ meV superimposed on the CDW state band structure of pristine sample ($h\nu = 49$ eV, LV-polarisation, $T = 18$ K).

measurements taken in the normal state of a more heavily doped Rb-dosed sample than the one shown in the main text. Supplementary Fig. S3(a,b) shows the corresponding measurements together with our fitted model for the normal-state electronic structure using the parameters listed in Table S1, but for $\Delta = 0$ and with the conduction bands displaced in momentum to be centered at the $TiSe_2$ M point and a rigid band shift of 52 meV to account for the finite electron doping. Note, there is a small overlap between the Ti $3d$ and Se $4p$ states. Adding a CDW hybridisation of $\Delta = 150$ meV yields the band structure shown in Supplementary Fig. S3(c), which is further modified by the moiré potential as described below.

TABLE S1. Effective model parameters

| $e_c$ | $\mu$ | $\nu$ | $e_h$ | $\mu_{inner}$ | $\mu_{outer}$ | $\lambda_{SOC}$ | $\Delta$ |
|---|---|---|---|---|---|---|---|
| $-0.058$ eV | $1.11$ eV $\cdot$ Å$^2$ | $12.15$ eV $\cdot$ Å$^2$ | $-0.143$ eV | $24.70$ eV $\cdot$ Å$^2$ | $12.10$ eV $\cdot$ Å$^2$ | $0.102$ eV | $0.150$ eV |

**Continuum model**

To include the moiré potential, we treat the problem perturbatively via a continuum approximation, in the spirit of the nearly free-electron model [61]. The Hamiltonian:

$$H = H_0(\mathbf{k}) + V(\mathbf{r}) \tag{S11}$$

with $V(\mathbf{r})$ representing the continuum intralayer moiré potential defined by the reciprocal lattice vector $\mathbf{q}$, where in our case $\mathbf{q} = \mathbf{q}_m^{\mathrm{CDW}}$ as defined in the main text. Starting from the unperturbed $H_0(\mathbf{k})$, solving the five-band model for a given $\mathbf{k}$ gives:

$$H_0(\mathbf{k})\psi_{i,\mathbf{k}}^{(0)} = \varepsilon_i^{(0)}(\mathbf{k})\psi_{i,\mathbf{k}}^{(0)} \tag{S12}$$

where the index $i$ refers to the five-band basis which diagonalize $H_0(\mathbf{k})$. By starting from the diagonalized basis, we consider only the main diagonal terms of the moiré potential, while we neglect second-order off-diagonal terms which would further mix conduction and valence bands. Using Bloch's theorem and expanding in terms of the moiré reciprocal vector:

$$\psi_{i,\mathbf{k}} = \sum_{\mathbf{q}} \alpha_{i,\mathbf{k}-\mathbf{q}} \psi_{i,\mathbf{k}-\mathbf{q}}^{(0)} = \sum_{\mathbf{q}} \alpha_{i,\mathbf{k}-\mathbf{q}} u(\mathbf{r}) e^{i(\mathbf{k}-\mathbf{q})\cdot\mathbf{r}} \tag{S13}$$

where we are already considering the need to work within the degenerate case. By using the Fourier expansion of the perturbative potential as: $V(\mathbf{r}) = \sum_{\mathbf{K}'} V_{\mathbf{K}'} e^{i\mathbf{K}'\cdot\mathbf{r}}$, substituting back into Eq. S11:

$$\sum_{\mathbf{q}} \psi_{i,\mathbf{k}-\mathbf{q}}^{(0)} \left( \varepsilon_i^{(0)}(\mathbf{k}-\mathbf{q})\alpha_{i,\mathbf{k}-\mathbf{q}} + \sum_{\mathbf{K}'} V_{\mathbf{K}'} \alpha_{i,\mathbf{k}-\mathbf{q}-\mathbf{K}'} \right) = \sum_{\mathbf{q}} \psi_{i,\mathbf{k}-\mathbf{q}}^{(0)} \varepsilon_i(\mathbf{k}). \tag{S14}$$

Setting $\mathbf{K}' \to \mathbf{K}' - \mathbf{q}$, we get the linear expression for each $i$-th band coefficient $\alpha^i$:

$$\sum_{\mathbf{q}} \psi^{(0)}_{i,\mathbf{k}-\mathbf{q}} \left( \left( \varepsilon^{(0)}_i(\mathbf{k}-\mathbf{q}) - \varepsilon_i(\mathbf{k}) \right) \alpha_{i,\mathbf{k}-\mathbf{q}} + \sum_{\mathbf{K}'} V_{i,\mathbf{K}'-\mathbf{q}} \alpha_{\mathbf{k}-\mathbf{K}'} \right) = 0. \tag{S15}$$

Each $i$-th state of the effective five-band model can then be treated independently, yielding a matrix which connects the states shifted by the reciprocal lattice $\mathbf{q}$. Writing explicitly the matrix equation for a few $\mathbf{q}$ vectors:

$$\det \begin{bmatrix} \ddots & & & & \\ & \varepsilon_i(\mathbf{k}) - \varepsilon^{(0)}_i(\mathbf{k}+\mathbf{2q}) & V_q & V_{2q} & V_{3q} \\ & V^*_q & \varepsilon_i(\mathbf{k}) - \varepsilon^{(0)}_i(\mathbf{k}+\mathbf{q}) & V_q & V_{2q} \\ & V_2q^* & V^*_q & \varepsilon_i(\mathbf{k}) - \varepsilon^{(0)}_i(\mathbf{k}) & V_g \\ & V^*_{3q} & V^*_{2q} & V^*_q & \varepsilon_i(\mathbf{k}) - \varepsilon^{(0)}_i(\mathbf{k}-\mathbf{q}) \\ & & & & \ddots \end{bmatrix} = 0. \tag{S16}$$

In the present case, the moiré potential takes into account only the first harmonic:

$$V(\mathbf{r}) = \sum_{j=1,2,3} 2V_0 \cos\left(\mathbf{q}_j \cdot \mathbf{r} + \phi\right), \tag{S17}$$

where $\mathbf{q}_j$ is the $j$-th moiré reciprocal lattice vector [20,62,63]. The Fourier coefficients of the moiré potential can then be written as delta functions connecting neighbouring reciprocal lattices:

$$V_{\mathbf{K}'-\mathbf{q}} = V_0 e^{i\phi} \delta_{(\mathbf{K}'-\mathbf{q}),\mathbf{q}_j} \tag{S18}$$

Using Eq. S16, we can construct the matrix expression which includes the five bands of the effective model in the CDW state. The low-energy band reconstruction can be adequately described utilising only a few reciprocal lattice shells. In the present work, we have performed the calculations using five shells, totalling $n = 90$ reciprocal lattice vectors. We take a moiré potential strength $V_0 = 15$ meV, and a phase $\phi = \pi/2$.

To facilitate comparison to the experimental data, we project the reconstructed electronic structure onto the original eigenstate of the unperturbed effective model, as plotted in the main text and reproduced in Supplementary Fig. S4(c). For each of the $n$-bands, we can define the spectral weight as:

$$w_n = \sum_{i=0}^{4} \left| c^{\mathbf{q}=0}_{i,n\mathbf{k}} \right|^2 \tag{S19}$$

where $c^{\mathbf{q}=0}_{i,n\mathbf{k}}$ is the element of each $n$-th $\mathbf{q}$ eigenvector resulting from the projection onto the original unit cell ($\mathbf{q} = 0$). From this, we simulate the spectral function $A(\mathbf{k}, \varepsilon)$:

$$A(\mathbf{k}, \varepsilon) = \sum_n \frac{w_n}{\pi^2} \frac{\gamma_e + \beta\varepsilon^2}{(\varepsilon - \varepsilon_n)^2 + (\gamma_e + \beta\varepsilon^2)^2}, \tag{S20}$$

in which we assumed a Fermi liquid-like (quadratic) imaginary part of the self-energy to take into account the energy-dependent broadening observed experimentally [64]. For the calculations shown in Fig. 3(h) of the main text, we take $\gamma = 0.015$ eV and $\beta = 0.10$ eV$^{-1}$.

### Band overlap and band flattening behaviour

The starting effective model in the CDW phase plays a significant role in the band flattening behaviour. In Supplementary Fig S4, we show a comparison between the model with parameters presented Table S1 (Supplementary Fig S4(a-d)) and one with a larger normal-state band overlap as given in Table S2 (Supplementary Fig S4(e-h)). For the second model, we have increased the energy overlap by adjusting the energy offset $e_h$ and the outer hole parameter $\mu_{outer}$. The $\lambda_{SOC}$ and $\Delta$ were also modified to give comparable band gap and SOC splitting of the valence bands in the CDW state. From the comparison of the results in the CDW state between the first (Supplementary Fig S4(b)) and second model (Supplementary Fig S4(f)) we note that the band overlap plays a significant role in the flattening of the valence band top due to the hybridisation introduced by the CDW. The

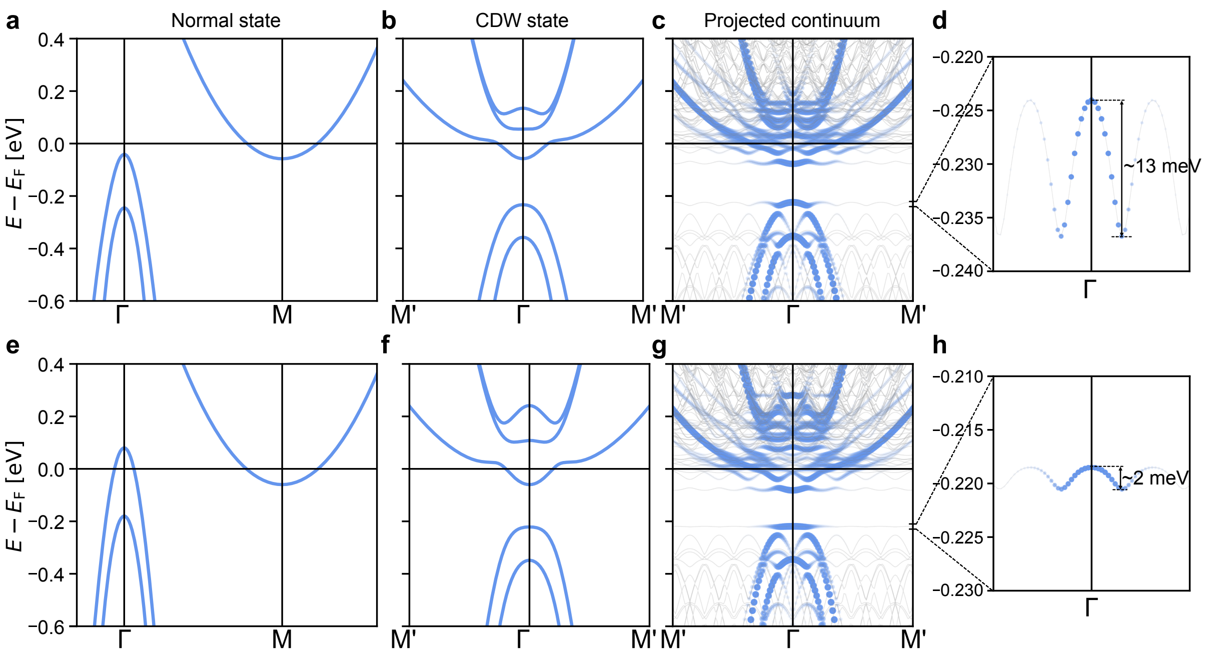


Supplementary Fig. S4. **Dependence of the electronic structure on normal-state band overlap.** (a) Normal state version of the five band model in Eq. S5 estimated from the more heavily doped Rb-dosed sample (parameters given in Table S1 with $\Delta = 0$, as also presented in Supplementary Fig. S3. (b) Corresponding CDW state calculation acquired by setting $\Delta = 0.150$ eV. (c) Continuum model calculations based in the calculations in (b) with $V_0 = 15$ meV and $\phi = \pi/2$, projected onto the original cell as described in the text. (d) Zoomed in image of the continuum model calculation displaying the top of the valence band featuring the flat band with an $\approx 11$ meV bandwidth. (e) Normal state version of the five band model with a larger band overlap, calculated using the parameters shown in Table S2. (f) CDW state calculation acquired by setting $\Delta = 0.180$ eV. (g) Corresponding projected continuum model, with $V_0 = 15$ meV and $\phi = \pi/2$. (h) Zoomed in image of the valence flat band with an estimated $\approx 2$ meV bandwidth.

projected continuum model acquired by setting the moiré potential $V_0 = 15$ meV and phase $\phi = \pi/2$ is shown in Supplementary Fig S4(c) and (g). While the major features are qualitatively similar in both calculations, the flattening behaviour of the valence band top is enhanced for the calculations starting from a larger normal-state band overlap, as shown in Supplementary Fig S4(d) and (h). From the estimated bandwidth of $\approx 13$ meV of the first model, a more significant band flattening behaviour is observed for the second model with a bandwidth of $\approx 2$ meV, in good agreement with our experimental measurements shown in the main text.

TABLE S2. Effective model parameters yielding a slightly larger band overlap in the normal state as compared to those in Table S1.

| $e_c$ | $\mu$ | $\nu$ | $e_h$ | $\mu_{inner}$ | $\mu_{outer}$ | $\lambda_{SOC}$ | $\Delta$ |
|---|---|---|---|---|---|---|---|
| −0.065 eV | 1.11 eV · Å$^2$ | 12.15 eV · Å$^2$ | −0.030 eV | 24.70 eV · Å$^2$ | 16.00 eV · Å$^2$ | 0.130 eV | 0.190 eV |
